# Supplementary material for: AdsorbDiff: Adsorbate Placement via Conditional Denoising Diffusion
Source: arXiv:2405.03962 source file (2024-05-07)
Supplement: Supplementary file 2 [file case_studies.tex]

\section{Case Studies}
\label{app:case_studies}
